# Supplementary material for: From AC-STEM Image to 3D Structure: A Systematic Analysis of Au55 nanocluster
Source: arXiv:2105.04270 ancillary file (2021-05-10)
Supplement: Supplementary file 1 [file SupportingInformation_Au55.pdf]

# Supporting Information (SI)
# From AC-STEM Image to 3D Structure: A Systematic Analysis of $Au_{55}$ nanocluster

Kusse S. Bersha,[†] Alejandro Peña-Torres,[†] and Hannes Jónsson[*,‡,¶]

†*Science Institute of the University of Iceland, 107 Reykjavík, Iceland*

‡*Faculty of Physical Sciences, University of Iceland, 107 Reykjavík, Iceland*

¶*Department of Applied Physics, Aalto University, FI-00076 Espoo, Finland*

E-mail: hj@hi.is

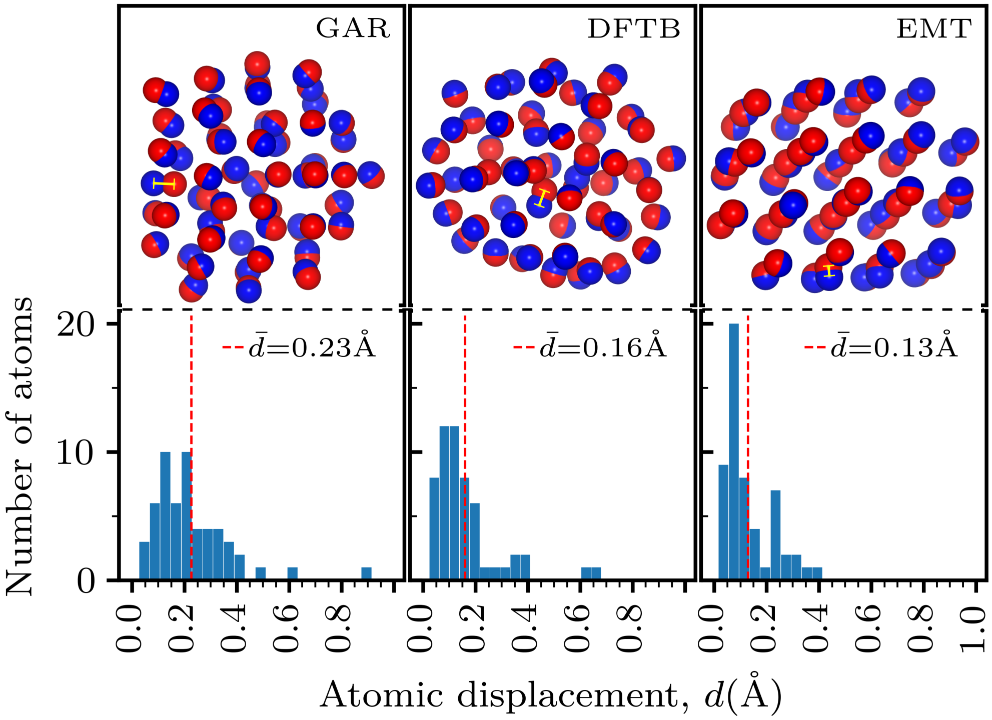


Figure S1: Atomic displacements during energy minimization at the DFT/PBEsol level starting with the Garzón, DFTB and EMT cluster structures. The yellow line segment indicates the largest displacement for each of the structures. The red dashed lines indicate the average displacement in each case.

Table S1: Relative abundance of selected CNA pairs (in %) for the structures generated in this study, as well as Garzón, icosahedron and cuboctahedron locally minimized with DFT/PBEsol. Indices with small relative abundance, such as 444, are ignored.

| CNA index | S1 | S2 | S3 | S4 | S5 | S6 | S7 | S8 | S9 | S10 | S11 |
|---|---|---|---|---|---|---|---|---|---|---|---|
| 211 | 2.75 | 3.43 | 9.13 | 3.3 | 3.76 | 2.34 | 4.61 | 1.41 | 2.39 | 2.39 | 3.37 |
| 311 | 30.73 | 26.47 | 28.37 | 31.13 | 30.52 | 30.37 | 28.57 | 31.46 | 28.71 | 26.79 | 26.44 |
| 322 | 23.85 | 22.06 | 12.02 | 20.75 | 17.37 | 21.5 | 19.35 | 20.19 | 25.36 | 20.57 | 20.67 |
| 421 | 1.83 | 0.98 | 6.25 | 4.25 | 0.47 | 2.34 | 2.76 | 1.41 | 0.48 | 2.87 | 3.37 |
| 422 | 17.43 | 7.35 | 6.25 | 13.68 | 12.68 | 16.36 | 21.2 | 16.9 | 6.7 | 11.0 | 6.73 |
| 433 | 5.96 | 4.41 | 9.13 | 3.77 | 7.98 | 3.74 | 3.69 | 4.23 | 8.61 | 5.74 | 7.69 |
| 544 | 2.29 | 1.96 | 3.37 | 2.83 | 3.76 | 1.87 | 2.76 | 1.88 | 1.91 | 1.91 | 2.88 |
| 555 | 3.67 | 2.94 | 0.48 | 2.36 | 2.35 | 3.27 | 3.69 | 3.29 | 3.35 | 2.87 | 2.4 |

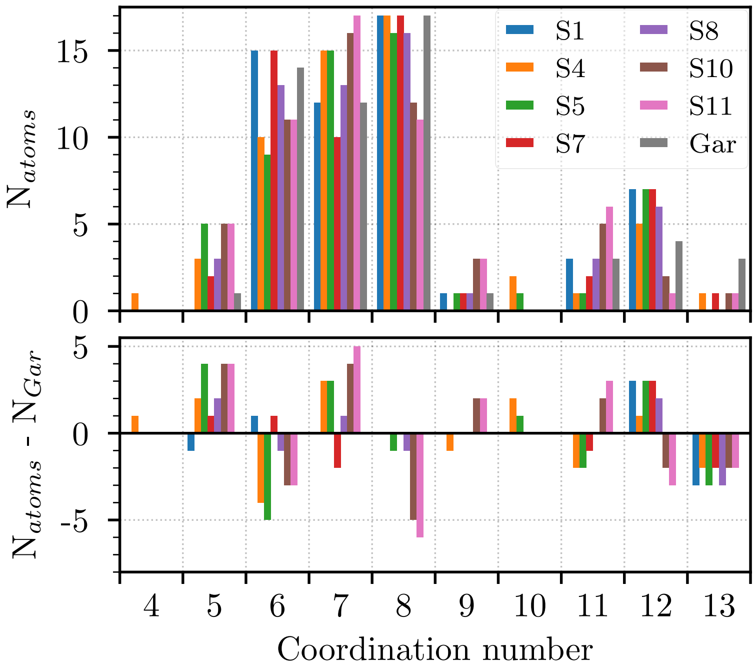


Figure S2: Top: Coordination numbers for several $Au_{55}$ cluster structures after minimization at the DFT/PBEsol level. Vertical axis shows number of atoms found with each coordination number. The cutoff distance for defining neighbors ('bonds') is 3.3 Å. Bottom: Differences in the coordination numbers with respect to the Garzón structure.

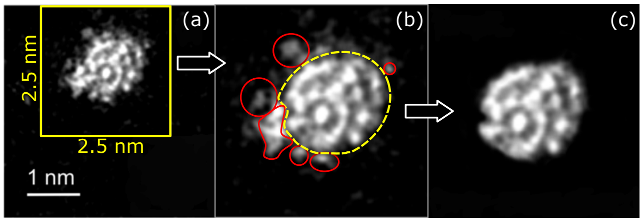


Figure S3: (a) Experimental AC-STEM image for $Au_{55}$ from Wang & Palmer. (b) Cropped image. Noise can be seen in the vicinity of the cluster, as indicated by red circles. (c) Image used in the fitting process, with noise removed.

Cartesian coordinates (in Å) of structures **S1-S11** and the DFT/PBEsol energy (in eV)

| **Structure S1 (E=-180.315 eV)** | | | |
|---|---|---|---|
| Au | 9.226089 | 9.685489 | 15.943182 |
| Au | 10.941731 | 11.787704 | 16.596160 |
| Au | 10.271347 | 14.317049 | 15.761490 |
| Au | 12.017902 | 16.380770 | 15.818449 |
| Au | 12.728290 | 13.925742 | 16.990574 |
| Au | 12.466897 | 12.872145 | 14.433898 |
| Au | 15.381088 | 13.343159 | 16.332625 |
| Au | 13.625285 | 11.318708 | 16.830057 |
| Au | 14.052140 | 15.043020 | 14.308963 |
| Au | 16.711099 | 15.479811 | 15.199118 |
| Au | 15.296770 | 17.389587 | 13.785712 |
| Au | 14.533447 | 15.980111 | 16.799427 |
| Au | 15.293048 | 11.399677 | 10.337747 |
| Au | 15.742883 | 8.443017 | 13.963032 |
| Au | 13.753818 | 10.479330 | 14.058780 |
| Au | 14.461293 | 9.124410 | 11.675103 |
| Au | 10.301665 | 8.081424 | 13.901154 |
| Au | 13.033625 | 7.802832 | 13.964188 |
| Au | 10.859977 | 10.753003 | 13.871985 |
| Au | 11.850015 | 9.183871 | 16.079322 |
| Au | 16.460752 | 15.245590 | 12.474308 |
| Au | 16.134209 | 10.846518 | 15.489294 |
| Au | 14.467603 | 8.788587 | 16.301807 |
| Au | 14.772550 | 12.839626 | 12.787017 |
| Au | 17.166995 | 13.002954 | 14.177074 |
| Au | 16.588514 | 10.650806 | 12.721567 |
| Au | 17.275119 | 12.910722 | 11.407758 |
| Au | 8.103613 | 10.021292 | 13.502833 |
| Au | 8.610175 | 12.217829 | 15.113242 |
| Au | 11.828444 | 8.485825 | 11.591795 |
| Au | 9.052715 | 8.451558 | 11.472778 |
| Au | 13.066391 | 10.041130 | 9.508245 |
| Au | 12.562229 | 11.510541 | 11.801049 |
| Au | 13.628989 | 12.651467 | 8.642758 |
| Au | 15.250075 | 14.225256 | 10.144726 |
| Au | 10.560527 | 9.052648 | 9.274995 |
| Au | 12.594136 | 14.460767 | 12.108960 |
| Au | 14.321313 | 16.535998 | 11.333441 |
| Au | 11.243770 | 11.360265 | 7.950554 |
| Au | 12.846446 | 15.383692 | 9.408409 |
| Au | 11.660833 | 14.050695 | 7.437205 |
| Au | 11.145953 | 13.209839 | 10.144932 |
| Au | 9.765830 | 15.351073 | 9.179053 |
| Au | 7.222458 | 10.559274 | 10.984759 |
| Au | 9.899854 | 11.071968 | 11.240808 |
| Au | 8.610164 | 10.790185 | 8.684780 |
| Au | 8.022189 | 13.178852 | 10.082393 |
| Au | 9.153260 | 13.190557 | 7.640243 |
| Au | 12.622003 | 17.313119 | 13.324429 |
| Au | 10.174424 | 16.293803 | 13.775581 |
| Au | 8.027105 | 14.755192 | 14.263169 |
| Au | 10.170426 | 13.328829 | 12.866187 |
| Au | 7.427413 | 12.664935 | 12.667520 |
| Au | 8.636584 | 15.313349 | 11.655692 |
| Au | 11.089100 | 16.599153 | 11.185947 |

**Structure S2 (E=-180.928 eV)**

| | | | |
|---|---|---|---|
| Au | 13.033630 | 17.243630 | 14.070868 |
| Au | 10.402609 | 16.496958 | 13.552802 |
| Au | 7.480253 | 12.346388 | 12.189154 |
| Au | 8.126729 | 14.877412 | 13.008531 |
| Au | 14.047717 | 12.407348 | 15.937885 |
| Au | 12.775878 | 11.936141 | 13.251414 |
| Au | 15.599610 | 11.103886 | 14.038063 |
| Au | 16.045970 | 13.768354 | 14.693940 |
| Au | 15.651967 | 16.465993 | 14.308169 |
| Au | 12.270121 | 13.847501 | 17.535798 |
| Au | 14.043235 | 15.157872 | 15.967654 |
| Au | 13.268563 | 14.730473 | 13.155710 |
| Au | 11.512921 | 16.110975 | 16.061735 |
| Au | 9.019557 | 15.252948 | 15.545934 |
| Au | 7.352306 | 10.392825 | 14.016397 |
| Au | 10.041517 | 11.512247 | 13.586729 |
| Au | 11.185091 | 8.753320 | 15.999367 |
| Au | 9.664840 | 13.083575 | 17.059663 |
| Au | 11.377898 | 13.553032 | 14.943571 |
| Au | 9.435257 | 8.690124 | 13.988664 |
| Au | 7.899669 | 12.886831 | 14.913703 |
| Au | 11.744973 | 11.254113 | 16.820463 |
| Au | 9.166024 | 10.599870 | 16.066581 |
| Au | 14.498570 | 8.955974 | 12.696871 |
| Au | 12.069589 | 8.052721 | 13.506424 |
| Au | 13.411045 | 9.879584 | 15.057561 |
| Au | 16.352728 | 15.578827 | 9.911118 |
| Au | 15.052580 | 13.060253 | 12.016584 |
| Au | 17.664370 | 12.465992 | 12.867527 |
| Au | 14.791322 | 16.767061 | 11.794488 |
| Au | 15.028481 | 13.757084 | 8.463172 |
| Au | 17.003845 | 15.060972 | 12.434695 |
| Au | 12.111518 | 16.836686 | 11.440804 |
| Au | 13.676058 | 10.969165 | 10.861582 |
| Au | 15.100459 | 8.682222 | 9.991300 |
| Au | 16.478202 | 10.507895 | 11.434430 |
| Au | 15.589687 | 11.093192 | 8.807518 |
| Au | 17.085595 | 12.970637 | 10.186283 |
| Au | 13.567088 | 11.900254 | 7.186907 |
| Au | 11.064264 | 11.763697 | 8.241381 |
| Au | 12.353368 | 14.216997 | 7.833187 |
| Au | 12.869866 | 13.661596 | 10.497813 |
| Au | 13.782995 | 16.087320 | 9.340095 |
| Au | 9.518356 | 16.078164 | 10.964832 |
| Au | 11.174135 | 16.446868 | 8.892039 |
| Au | 12.947603 | 9.679933 | 8.521670 |
| Au | 10.388992 | 9.432926 | 9.536808 |
| Au | 11.041385 | 11.583806 | 11.066415 |
| Au | 8.576789 | 9.895934 | 11.596633 |
| Au | 7.631768 | 14.256153 | 10.350894 |
| Au | 9.825106 | 14.121038 | 8.820126 |
| Au | 10.715331 | 13.984750 | 12.312228 |
| Au | 8.684559 | 11.802706 | 9.685731 |
| Au | 10.112845 | 7.670344 | 11.610278 |
| Au | 12.581714 | 8.212800 | 10.817525 |

**Structure S3 (E=-180.347 eV)**

| | | | |
|---|---|---|---|
| Au | 16.797689 | 10.148884 | 13.063523 |
| Au | 15.580699 | 11.181524 | 10.718153 |
| Au | 12.949611 | 12.203246 | 11.720730 |
| Au | 17.554007 | 12.576324 | 11.946319 |
| Au | 15.124700 | 12.258689 | 13.342435 |
| Au | 17.399871 | 13.377715 | 14.528883 |
| Au | 16.371962 | 11.166598 | 15.655176 |
| Au | 12.668421 | 12.395651 | 14.541258 |
| Au | 13.866348 | 16.054552 | 16.069406 |
| Au | 12.545778 | 13.743842 | 16.958349 |
| Au | 15.152784 | 13.562123 | 16.234810 |
| Au | 16.327958 | 15.790699 | 15.087440 |
| Au | 10.609129 | 10.828551 | 11.053730 |
| Au | 9.468037 | 8.278970 | 11.414836 |
| Au | 9.609804 | 9.238839 | 15.940932 |
| Au | 8.401940 | 11.641816 | 15.568672 |
| Au | 8.362343 | 9.603196 | 13.587060 |
| Au | 10.217702 | 11.699069 | 13.553576 |
| Au | 11.046296 | 11.437590 | 16.615237 |
| Au | 9.881812 | 13.853628 | 16.312305 |
| Au | 12.286114 | 9.046883 | 15.787717 |
| Au | 12.422562 | 9.990248 | 13.187442 |
| Au | 14.709023 | 9.293745 | 14.676714 |
| Au | 10.689995 | 7.951519 | 13.811601 |
| Au | 14.666649 | 8.856884 | 11.983044 |
| Au | 12.175726 | 7.915447 | 11.437107 |
| Au | 10.923111 | 8.842849 | 9.151751 |
| Au | 13.293315 | 9.964926 | 9.874927 |
| Au | 13.830460 | 11.143926 | 16.663438 |
| Au | 13.990686 | 14.655625 | 13.687045 |
| Au | 13.943475 | 12.533226 | 8.973844 |
| Au | 12.964104 | 17.528753 | 11.368176 |
| Au | 14.262814 | 15.278515 | 8.495166 |
| Au | 15.428929 | 16.580644 | 10.615712 |
| Au | 16.004045 | 13.887182 | 10.150283 |
| Au | 11.260647 | 16.146751 | 16.488002 |
| Au | 12.200764 | 16.909805 | 13.962199 |
| Au | 14.874892 | 17.192824 | 13.275499 |
| Au | 16.760084 | 15.152314 | 12.481495 |
| Au | 11.711653 | 16.221644 | 9.308017 |
| Au | 13.368292 | 14.774123 | 11.043622 |
| Au | 10.456449 | 16.572570 | 11.753159 |
| Au | 9.678071 | 15.925567 | 14.336308 |
| Au | 11.302102 | 14.193336 | 12.905209 |
| Au | 8.453601 | 14.697312 | 12.215330 |
| Au | 7.700629 | 14.145942 | 14.775976 |
| Au | 8.957118 | 10.702899 | 8.737603 |
| Au | 9.123573 | 15.375423 | 9.645730 |
| Au | 9.453382 | 13.244212 | 7.936180 |
| Au | 8.032985 | 12.872707 | 10.273466 |
| Au | 7.501690 | 12.207967 | 12.930971 |
| Au | 7.693092 | 10.287713 | 11.058857 |
| Au | 12.023762 | 14.033947 | 7.671477 |
| Au | 11.562053 | 11.385052 | 8.244940 |
| Au | 10.960479 | 13.459841 | 10.279803 |

**Structure S4 (E=-179.386 eV)**

| | | | |
|---|---|---|---|
| Au | 14.781271 | 16.331911 | 13.299680 |
| Au | 15.211182 | 13.488051 | 8.217268 |
| Au | 16.376003 | 15.947037 | 8.643807 |
| Au | 16.315696 | 16.850542 | 11.190960 |
| Au | 14.229549 | 17.579093 | 9.560840 |
| Au | 14.291532 | 15.025611 | 10.507790 |
| Au | 11.937845 | 16.068362 | 9.105728 |
| Au | 12.483352 | 12.971185 | 10.258744 |
| Au | 12.470989 | 13.640156 | 7.563019 |
| Au | 13.994678 | 15.818540 | 7.399822 |
| Au | 10.965601 | 11.493397 | 8.317676 |
| Au | 14.639095 | 8.527737 | 13.939360 |
| Au | 15.794224 | 9.929699 | 11.923021 |
| Au | 17.160293 | 12.288629 | 12.612316 |
| Au | 14.652489 | 12.627066 | 11.799012 |
| Au | 17.264466 | 15.021038 | 12.895106 |
| Au | 15.232181 | 11.190699 | 14.284757 |
| Au | 15.452421 | 13.888407 | 14.426417 |
| Au | 11.939737 | 8.112199 | 13.841654 |
| Au | 13.092575 | 9.998370 | 15.556697 |
| Au | 12.587655 | 11.714134 | 13.348303 |
| Au | 13.538034 | 12.692734 | 15.886355 |
| Au | 14.883556 | 9.151441 | 9.475569 |
| Au | 16.189264 | 11.470922 | 9.731246 |
| Au | 13.366503 | 8.444335 | 11.566678 |
| Au | 13.720959 | 11.244544 | 8.240341 |
| Au | 12.198057 | 9.132409 | 9.209374 |
| Au | 10.626848 | 8.123570 | 11.446183 |
| Au | 16.958416 | 13.966452 | 10.410862 |
| Au | 10.889564 | 13.560733 | 14.674369 |
| Au | 11.327111 | 16.841285 | 16.411741 |
| Au | 13.347949 | 15.407359 | 15.364417 |
| Au | 9.210975 | 13.262691 | 17.269347 |
| Au | 11.729092 | 14.265105 | 17.240702 |
| Au | 10.967210 | 16.388320 | 13.768922 |
| Au | 10.209077 | 15.943774 | 11.147645 |
| Au | 10.256901 | 13.232737 | 11.951413 |
| Au | 8.011074 | 14.469287 | 10.495999 |
| Au | 8.608332 | 11.898086 | 9.758526 |
| Au | 8.480171 | 15.043835 | 13.111808 |
| Au | 7.487872 | 12.472537 | 12.224124 |
| Au | 7.893975 | 13.070563 | 14.882060 |
| Au | 9.136107 | 15.465076 | 15.694859 |
| Au | 10.655480 | 8.997538 | 16.030946 |
| Au | 7.285269 | 10.474697 | 14.012996 |
| Au | 8.677973 | 10.790601 | 16.292796 |
| Au | 9.986591 | 11.093810 | 13.779508 |
| Au | 9.204283 | 8.448826 | 13.784242 |
| Au | 11.272682 | 11.550128 | 16.866112 |
| Au | 9.523540 | 9.365242 | 9.232071 |
| Au | 8.314476 | 9.854039 | 11.582531 |
| Au | 11.168383 | 10.758005 | 11.227559 |
| Au | 12.634743 | 17.073604 | 11.708765 |
| Au | 12.689940 | 14.451393 | 12.697857 |
| Au | 10.135475 | 14.056083 | 8.921808 |

**Structure S5 (E=-180.613 eV)**

| | | | |
|---|---|---|---|
| Au | 15.682824 | 11.196985 | 15.797393 |
| Au | 15.739812 | 13.754344 | 15.124076 |
| Au | 13.276269 | 14.475268 | 13.159139 |
| Au | 12.770986 | 11.665592 | 12.654615 |
| Au | 13.102606 | 17.170591 | 13.669308 |
| Au | 11.384852 | 16.787062 | 15.707427 |
| Au | 11.403550 | 14.404605 | 17.081318 |
| Au | 13.753655 | 12.786781 | 16.911777 |
| Au | 13.660098 | 15.331225 | 15.887147 |
| Au | 13.176104 | 10.263780 | 15.836048 |
| Au | 11.150823 | 11.559587 | 17.192725 |
| Au | 7.881992 | 12.944279 | 14.485828 |
| Au | 10.486364 | 16.530533 | 13.100025 |
| Au | 9.375251 | 15.112324 | 15.117967 |
| Au | 8.981721 | 13.264122 | 17.014400 |
| Au | 8.662540 | 10.804334 | 16.069222 |
| Au | 11.934917 | 12.846699 | 14.909820 |
| Au | 10.733840 | 9.171697 | 15.868621 |
| Au | 12.193663 | 8.869219 | 13.630012 |
| Au | 9.439613 | 8.474489 | 13.568185 |
| Au | 7.411154 | 10.341795 | 13.739776 |
| Au | 10.163462 | 11.111549 | 13.613454 |
| Au | 8.402245 | 9.734474 | 11.313649 |
| Au | 7.720235 | 14.219940 | 9.997185 |
| Au | 10.523767 | 13.685670 | 12.757361 |
| Au | 9.812076 | 15.784614 | 10.593319 |
| Au | 8.146815 | 14.946439 | 12.615227 |
| Au | 7.556859 | 12.303998 | 11.851894 |
| Au | 12.221063 | 13.848295 | 10.541394 |
| Au | 14.123489 | 15.588680 | 9.215236 |
| Au | 16.568481 | 11.004462 | 8.685254 |
| Au | 15.343800 | 13.324124 | 8.378775 |
| Au | 16.632673 | 15.032893 | 10.056605 |
| Au | 17.376620 | 12.507005 | 10.769940 |
| Au | 12.709574 | 13.558462 | 7.773818 |
| Au | 14.963088 | 16.381325 | 11.713823 |
| Au | 13.913548 | 11.101833 | 7.463902 |
| Au | 15.965803 | 10.180508 | 11.243819 |
| Au | 14.892687 | 8.979042 | 8.995042 |
| Au | 13.619224 | 8.724216 | 11.362936 |
| Au | 11.125081 | 11.337108 | 8.022079 |
| Au | 12.243469 | 8.944471 | 8.894571 |
| Au | 13.307019 | 11.281418 | 10.054571 |
| Au | 10.894442 | 8.468973 | 11.252600 |
| Au | 14.738210 | 9.850928 | 13.620583 |
| Au | 16.851304 | 14.500977 | 12.726035 |
| Au | 14.800306 | 13.146783 | 11.361421 |
| Au | 16.609155 | 11.843747 | 13.330397 |
| Au | 15.617166 | 16.336129 | 14.314020 |
| Au | 12.349406 | 16.698283 | 11.081216 |
| Au | 8.396797 | 11.669389 | 9.271982 |
| Au | 9.608874 | 9.272376 | 8.954782 |
| Au | 11.561261 | 15.947068 | 8.544621 |
| Au | 10.031267 | 13.738644 | 8.624706 |
| Au | 10.612271 | 11.529341 | 10.878500 |

**Structure S6 (E=-180.872 eV)**

| | | | |
|---|---|---|---|
| Au | 9.170846 | 9.776198 | 16.192163 |
| Au | 10.907121 | 11.906244 | 16.879610 |
| Au | 10.386876 | 14.404987 | 15.891121 |
| Au | 12.432158 | 16.082000 | 15.312979 |
| Au | 12.707157 | 14.004404 | 17.350548 |
| Au | 12.817635 | 12.938270 | 14.885948 |
| Au | 15.366292 | 13.248406 | 16.785054 |
| Au | 13.529500 | 11.334617 | 17.323589 |
| Au | 15.146126 | 12.678267 | 13.345371 |
| Au | 16.886723 | 15.236867 | 15.644973 |
| Au | 14.889401 | 16.325607 | 14.131572 |
| Au | 14.585433 | 15.850647 | 16.836667 |
| Au | 15.832591 | 10.985525 | 11.064265 |
| Au | 15.782876 | 8.201211 | 14.814838 |
| Au | 13.864421 | 10.417936 | 14.548127 |
| Au | 14.753974 | 8.806657 | 12.383886 |
| Au | 10.395849 | 8.174345 | 14.244589 |
| Au | 13.083708 | 7.742386 | 14.547276 |
| Au | 11.047791 | 10.856379 | 14.188072 |
| Au | 11.767410 | 9.277393 | 16.477804 |
| Au | 16.923242 | 14.844703 | 12.994034 |
| Au | 16.101251 | 10.675578 | 16.251704 |
| Au | 14.309139 | 8.747835 | 16.975658 |
| Au | 16.232616 | 13.659013 | 10.618379 |
| Au | 17.396171 | 12.686043 | 14.958242 |
| Au | 16.821419 | 10.286994 | 13.563161 |
| Au | 17.878923 | 12.378656 | 12.289778 |
| Au | 8.291462 | 10.076632 | 13.661023 |
| Au | 8.670065 | 12.278849 | 15.298795 |
| Au | 12.105885 | 8.342138 | 12.074417 |
| Au | 9.352401 | 8.456505 | 11.717899 |
| Au | 13.541957 | 9.825745 | 10.176309 |
| Au | 12.917562 | 11.599847 | 12.220159 |
| Au | 14.327711 | 12.302639 | 9.216796 |
| Au | 14.778166 | 15.021228 | 8.893741 |
| Au | 11.065768 | 8.931179 | 9.661541 |
| Au | 13.123057 | 14.426266 | 12.637316 |
| Au | 15.021722 | 16.047607 | 11.420680 |
| Au | 11.913030 | 11.291972 | 8.528763 |
| Au | 12.581784 | 16.034650 | 10.126871 |
| Au | 12.420999 | 14.039200 | 8.156073 |
| Au | 11.503316 | 13.355756 | 10.641354 |
| Au | 9.987754 | 15.281724 | 9.366920 |
| Au | 7.615206 | 10.527388 | 11.066835 |
| Au | 10.305735 | 11.061481 | 11.522713 |
| Au | 9.201413 | 10.678640 | 8.890146 |
| Au | 8.393614 | 13.048168 | 10.112746 |
| Au | 9.950889 | 13.053290 | 7.885525 |
| Au | 12.684946 | 17.103955 | 12.716073 |
| Au | 10.250965 | 16.300430 | 13.791117 |
| Au | 8.138219 | 14.756089 | 14.399430 |
| Au | 10.480284 | 13.412073 | 13.185736 |
| Au | 7.712971 | 12.658567 | 12.729913 |
| Au | 8.644076 | 15.158943 | 11.770289 |
| Au | 10.402478 | 17.165642 | 11.245904 |

**Structure S7 (E=-180.910 eV)**

| | | | |
|---|---|---|---|
| Au | 9.113162 | 10.434272 | 16.401313 |
| Au | 10.898786 | 12.410633 | 17.071781 |
| Au | 10.488132 | 14.928413 | 15.985704 |
| Au | 12.599276 | 16.523313 | 15.509890 |
| Au | 12.822210 | 14.424300 | 17.445794 |
| Au | 12.780175 | 13.236606 | 15.039497 |
| Au | 15.469061 | 13.480423 | 17.074140 |
| Au | 13.505510 | 11.660605 | 17.422134 |
| Au | 15.396192 | 12.864257 | 14.333061 |
| Au | 16.853796 | 15.085566 | 15.286453 |
| Au | 15.076041 | 16.807793 | 14.161033 |
| Au | 14.879986 | 16.092777 | 16.813377 |
| Au | 15.754137 | 9.628015 | 11.966528 |
| Au | 15.628800 | 8.658510 | 14.588126 |
| Au | 13.692858 | 10.605057 | 14.648099 |
| Au | 14.094160 | 7.554839 | 12.618063 |
| Au | 10.057777 | 8.543691 | 14.644606 |
| Au | 12.755970 | 7.896099 | 14.961125 |
| Au | 10.973686 | 11.191721 | 14.353789 |
| Au | 11.655809 | 9.689632 | 16.738251 |
| Au | 16.273114 | 14.971959 | 12.550920 |
| Au | 16.023305 | 10.943311 | 16.298252 |
| Au | 14.248811 | 9.008814 | 16.952210 |
| Au | 13.433627 | 12.285014 | 12.444730 |
| Au | 18.071681 | 13.245677 | 13.768624 |
| Au | 17.299495 | 10.678055 | 13.908597 |
| Au | 16.477381 | 12.268952 | 11.780193 |
| Au | 8.227143 | 10.593509 | 13.849192 |
| Au | 8.680098 | 12.887597 | 15.406099 |
| Au | 11.380759 | 7.171975 | 12.692364 |
| Au | 9.344391 | 8.915944 | 11.990184 |
| Au | 13.939141 | 8.707167 | 10.175948 |
| Au | 12.372399 | 9.754449 | 12.358969 |
| Au | 14.684025 | 11.294469 | 10.031497 |
| Au | 14.922252 | 14.044163 | 10.392036 |
| Au | 11.288522 | 8.296848 | 10.194368 |
| Au | 13.190753 | 14.996808 | 13.020346 |
| Au | 14.473743 | 16.628276 | 11.285286 |
| Au | 12.315564 | 10.484662 | 8.883727 |
| Au | 13.048608 | 15.646212 | 9.168872 |
| Au | 13.298078 | 13.018667 | 8.472007 |
| Au | 11.838475 | 13.770534 | 10.828839 |
| Au | 10.287716 | 15.254015 | 9.149571 |
| Au | 7.669000 | 10.948677 | 11.216010 |
| Au | 10.444433 | 11.589318 | 11.693784 |
| Au | 9.612218 | 10.300515 | 9.432144 |
| Au | 8.656432 | 13.235816 | 10.151739 |
| Au | 10.653423 | 12.610228 | 8.474212 |
| Au | 12.876651 | 17.921729 | 13.120626 |
| Au | 10.555054 | 16.712639 | 13.697292 |
| Au | 8.359498 | 15.322449 | 14.296402 |
| Au | 10.635903 | 13.851899 | 13.319584 |
| Au | 7.874690 | 13.169758 | 12.756982 |
| Au | 9.084767 | 15.525638 | 11.623333 |
| Au | 11.492876 | 16.786250 | 11.099082 |

**Structure S8 (E=-180.850 eV)**

| | | | |
|---|---|---|---|
| Au | 9.532962 | 9.092409 | 15.894313 |
| Au | 11.190049 | 11.243272 | 16.760883 |
| Au | 10.279712 | 13.750191 | 16.351031 |
| Au | 11.787248 | 15.951171 | 16.548845 |
| Au | 12.912322 | 13.538705 | 17.254847 |
| Au | 12.761224 | 12.662152 | 14.741694 |
| Au | 15.482664 | 13.093862 | 16.198725 |
| Au | 13.886418 | 10.965362 | 16.922660 |
| Au | 12.401743 | 16.875540 | 14.070977 |
| Au | 16.540986 | 14.894050 | 14.199451 |
| Au | 15.005491 | 16.978530 | 13.540037 |
| Au | 14.257515 | 15.424001 | 15.644815 |
| Au | 15.779056 | 11.343079 | 10.599960 |
| Au | 16.127742 | 8.272958 | 14.004907 |
| Au | 13.993044 | 10.276175 | 14.096517 |
| Au | 14.872608 | 9.021025 | 11.748087 |
| Au | 10.707553 | 7.809603 | 13.726763 |
| Au | 13.449171 | 7.588539 | 13.798804 |
| Au | 11.160102 | 10.527883 | 13.901494 |
| Au | 12.160320 | 8.783846 | 15.975268 |
| Au | 15.810415 | 15.363678 | 11.555912 |
| Au | 16.359913 | 10.509525 | 15.704900 |
| Au | 14.742056 | 8.418502 | 16.301676 |
| Au | 15.078058 | 12.719591 | 13.238726 |
| Au | 17.698906 | 12.536787 | 14.623978 |
| Au | 16.973567 | 10.553729 | 12.883850 |
| Au | 17.452838 | 13.173531 | 11.988422 |
| Au | 8.427171 | 9.662052 | 13.486977 |
| Au | 8.774126 | 11.606596 | 15.405603 |
| Au | 12.244015 | 8.377250 | 11.484258 |
| Au | 9.505733 | 8.404037 | 11.339495 |
| Au | 13.465993 | 10.145149 | 9.726055 |
| Au | 12.893048 | 11.756109 | 11.939498 |
| Au | 14.286572 | 12.491038 | 8.660801 |
| Au | 16.512890 | 13.715040 | 9.525211 |
| Au | 10.967395 | 9.230570 | 9.232033 |
| Au | 13.000581 | 14.477234 | 12.727105 |
| Au | 13.400252 | 16.788457 | 11.352196 |
| Au | 11.741786 | 11.629005 | 8.200220 |
| Au | 14.295339 | 15.233077 | 9.289190 |
| Au | 12.497538 | 14.154834 | 7.580500 |
| Au | 11.109972 | 13.658010 | 10.854398 |
| Au | 9.020514 | 15.655988 | 9.971556 |
| Au | 7.654956 | 10.422564 | 10.965958 |
| Au | 10.303406 | 11.107762 | 11.351693 |
| Au | 9.120277 | 11.146161 | 8.785196 |
| Au | 8.124909 | 13.105836 | 10.416195 |
| Au | 9.945397 | 13.708666 | 8.336306 |
| Au | 10.729947 | 16.364610 | 11.992294 |
| Au | 9.928064 | 15.888466 | 14.554598 |
| Au | 7.947208 | 14.107581 | 14.976509 |
| Au | 10.343344 | 13.163710 | 13.450262 |
| Au | 7.594733 | 12.270574 | 12.976181 |
| Au | 8.360190 | 14.932096 | 12.452060 |
| Au | 11.661095 | 15.947657 | 9.412857 |

**Structure S9 (E=-180.706 eV)**

| | | | |
|---|---|---|---|
| Au | 9.540219 | 9.207873 | 16.096029 |
| Au | 11.056889 | 11.246447 | 17.222336 |
| Au | 10.285343 | 13.690005 | 16.274590 |
| Au | 11.867353 | 15.823086 | 16.505016 |
| Au | 12.866880 | 13.377703 | 17.270970 |
| Au | 12.911604 | 13.501967 | 14.539015 |
| Au | 15.440147 | 12.986576 | 16.417688 |
| Au | 13.781356 | 10.815236 | 17.301476 |
| Au | 12.666555 | 16.688000 | 14.075967 |
| Au | 16.625833 | 14.616763 | 14.490751 |
| Au | 15.325554 | 16.883074 | 13.811306 |
| Au | 14.444788 | 15.443872 | 15.927987 |
| Au | 15.750322 | 10.558992 | 9.426448 |
| Au | 16.211923 | 9.253522 | 13.924117 |
| Au | 14.230337 | 11.028252 | 14.521898 |
| Au | 14.747206 | 9.250660 | 11.613306 |
| Au | 10.800629 | 8.173455 | 13.935981 |
| Au | 13.547714 | 8.237006 | 13.824234 |
| Au | 11.477268 | 10.996899 | 14.554437 |
| Au | 12.184541 | 8.812664 | 16.247397 |
| Au | 16.037426 | 15.433651 | 11.667887 |
| Au | 16.411731 | 10.482309 | 16.517564 |
| Au | 14.806179 | 8.400169 | 16.173232 |
| Au | 15.033571 | 13.035253 | 12.757237 |
| Au | 17.117105 | 11.902246 | 14.394415 |
| Au | 16.888282 | 10.933276 | 11.841300 |
| Au | 17.805037 | 13.476734 | 12.288922 |
| Au | 8.293066 | 9.598623 | 13.659214 |
| Au | 8.760674 | 11.652245 | 15.404477 |
| Au | 12.122308 | 8.485674 | 11.547366 |
| Au | 9.368339 | 8.058457 | 11.641805 |
| Au | 13.126267 | 10.027457 | 9.530259 |
| Au | 12.908520 | 11.496110 | 12.112491 |
| Au | 13.999464 | 12.450365 | 8.586638 |
| Au | 16.174205 | 13.110184 | 10.124935 |
| Au | 10.475623 | 9.406514 | 9.546199 |
| Au | 12.781519 | 14.392962 | 11.939374 |
| Au | 13.765034 | 16.974493 | 11.584282 |
| Au | 11.424400 | 11.521687 | 8.049079 |
| Au | 14.299169 | 14.996001 | 9.602308 |
| Au | 12.019722 | 14.247485 | 8.294116 |
| Au | 11.055227 | 12.821083 | 10.501675 |
| Au | 9.763146 | 15.321148 | 9.798809 |
| Au | 7.880634 | 10.294889 | 10.938218 |
| Au | 10.334492 | 10.687266 | 12.077623 |
| Au | 8.676632 | 11.019520 | 8.473000 |
| Au | 8.181113 | 13.038579 | 10.300226 |
| Au | 9.472731 | 13.479001 | 7.881621 |
| Au | 10.925707 | 16.536334 | 11.963170 |
| Au | 10.116730 | 15.816330 | 14.419960 |
| Au | 8.028257 | 14.160177 | 14.732219 |
| Au | 10.466350 | 13.217292 | 13.235798 |
| Au | 7.767138 | 12.229079 | 12.859563 |
| Au | 8.607155 | 14.971574 | 12.197520 |
| Au | 12.108432 | 16.645338 | 9.516991 |

**Structure S10 (E=-181.007 eV)**

| | | | |
|---|---|---|---|
| Au | 13.170841 | 16.962593 | 14.152539 |
| Au | 10.513718 | 16.322512 | 13.543515 |
| Au | 7.460493 | 12.278131 | 12.199254 |
| Au | 8.207507 | 14.845556 | 13.032285 |
| Au | 13.933838 | 12.334112 | 16.018833 |
| Au | 12.697794 | 11.892740 | 13.409755 |
| Au | 15.557416 | 10.989838 | 14.265158 |
| Au | 16.061650 | 13.631729 | 15.001283 |
| Au | 15.778779 | 16.320767 | 14.566760 |
| Au | 12.081790 | 13.746128 | 17.423564 |
| Au | 14.040367 | 15.083228 | 16.144930 |
| Au | 12.738913 | 14.619162 | 12.813428 |
| Au | 11.495771 | 16.027311 | 16.074280 |
| Au | 8.938034 | 15.246248 | 15.602946 |
| Au | 7.332719 | 10.248445 | 13.981091 |
| Au | 10.009123 | 11.246889 | 13.632831 |
| Au | 11.023508 | 8.640469 | 16.009373 |
| Au | 9.503781 | 12.975325 | 17.053172 |
| Au | 10.991496 | 13.574618 | 14.736599 |
| Au | 9.463266 | 8.512231 | 13.828315 |
| Au | 7.875373 | 12.799291 | 14.865136 |
| Au | 11.555938 | 11.190666 | 16.705034 |
| Au | 8.995040 | 10.447035 | 16.095892 |
| Au | 14.700418 | 8.703041 | 13.016670 |
| Au | 12.138881 | 7.807179 | 13.688198 |
| Au | 13.320227 | 9.769040 | 15.154996 |
| Au | 16.536537 | 15.447140 | 10.150929 |
| Au | 14.980258 | 13.107765 | 12.346454 |
| Au | 17.697596 | 12.278588 | 13.284684 |
| Au | 14.881626 | 16.503846 | 12.020872 |
| Au | 15.261826 | 13.469128 | 8.805955 |
| Au | 17.103817 | 14.885974 | 12.721818 |
| Au | 12.265995 | 16.983104 | 11.446988 |
| Au | 13.928596 | 10.719168 | 11.266536 |
| Au | 15.138983 | 8.673703 | 10.025055 |
| Au | 16.641738 | 10.271977 | 11.796178 |
| Au | 16.289487 | 10.940194 | 9.151732 |
| Au | 17.259297 | 12.893280 | 10.690924 |
| Au | 13.757008 | 11.262326 | 8.373540 |
| Au | 11.114996 | 11.565767 | 8.416686 |
| Au | 12.627768 | 13.881262 | 7.988882 |
| Au | 12.832316 | 13.093509 | 10.548109 |
| Au | 13.953820 | 15.767320 | 9.560503 |
| Au | 9.754389 | 16.020546 | 10.979860 |
| Au | 11.446538 | 16.265180 | 8.902996 |
| Au | 12.429645 | 9.097659 | 9.371585 |
| Au | 9.728777 | 9.344215 | 9.182420 |
| Au | 11.151338 | 10.859850 | 11.188811 |
| Au | 8.446410 | 9.737103 | 11.561983 |
| Au | 7.800083 | 14.251251 | 10.406456 |
| Au | 10.040225 | 14.004913 | 8.908916 |
| Au | 10.323637 | 13.406615 | 11.886789 |
| Au | 8.687349 | 11.782355 | 9.762365 |
| Au | 10.637899 | 8.043684 | 11.402391 |
| Au | 13.212719 | 7.279729 | 11.272334 |

**Structure S11 (E=-181.028 eV)**

| | | | |
|---|---|---|---|
| Au | 13.110550 | 16.994780 | 14.197441 |
| Au | 10.446069 | 16.440098 | 13.628778 |
| Au | 7.518945 | 12.293965 | 12.291119 |
| Au | 8.145062 | 14.906802 | 13.101237 |
| Au | 14.024876 | 12.386998 | 16.063379 |
| Au | 12.773113 | 12.023852 | 13.525475 |
| Au | 15.512111 | 11.109865 | 14.107128 |
| Au | 16.041319 | 13.735638 | 14.885595 |
| Au | 15.750626 | 16.434154 | 14.540474 |
| Au | 12.214924 | 13.789878 | 17.524885 |
| Au | 14.064486 | 15.148465 | 16.141200 |
| Au | 12.598778 | 14.701343 | 12.776727 |
| Au | 11.476208 | 16.003747 | 16.147274 |
| Au | 8.893677 | 15.332821 | 15.662651 |
| Au | 7.346598 | 10.346924 | 14.122503 |
| Au | 10.070396 | 11.275878 | 13.770886 |
| Au | 11.116536 | 8.720767 | 16.138876 |
| Au | 9.628334 | 13.097888 | 17.106146 |
| Au | 10.936286 | 13.671995 | 14.732088 |
| Au | 9.373978 | 8.554139 | 14.122381 |
| Au | 7.901137 | 12.871667 | 14.976108 |
| Au | 11.667085 | 11.250830 | 16.841871 |
| Au | 9.074182 | 10.552525 | 16.233198 |
| Au | 14.570645 | 8.784048 | 12.956682 |
| Au | 12.052617 | 7.966481 | 13.693201 |
| Au | 13.364977 | 9.840404 | 15.193469 |
| Au | 16.404585 | 15.487901 | 10.140619 |
| Au | 14.917599 | 13.402030 | 12.216825 |
| Au | 17.623171 | 12.428856 | 13.080098 |
| Au | 14.783726 | 16.570495 | 12.027116 |
| Au | 15.113664 | 13.674588 | 8.661770 |
| Au | 17.115862 | 15.047597 | 12.672934 |
| Au | 12.152831 | 17.090211 | 11.502647 |
| Au | 14.020656 | 10.943561 | 11.292757 |
| Au | 15.199881 | 8.575309 | 10.243627 |
| Au | 16.676688 | 10.336312 | 11.678724 |
| Au | 15.669475 | 10.978808 | 9.022038 |
| Au | 17.032094 | 12.854352 | 10.466638 |
| Au | 13.698797 | 11.831728 | 7.350204 |
| Au | 11.232398 | 11.704097 | 8.454763 |
| Au | 12.487971 | 14.218778 | 7.871796 |
| Au | 12.775995 | 13.241168 | 10.423151 |
| Au | 13.825131 | 15.960622 | 9.551556 |
| Au | 9.639230 | 16.088383 | 11.071729 |
| Au | 11.274845 | 16.458200 | 8.967069 |
| Au | 13.084729 | 9.686294 | 8.821436 |
| Au | 10.407526 | 9.282662 | 9.553208 |
| Au | 11.327851 | 10.976582 | 11.385140 |
| Au | 8.560072 | 9.781748 | 11.711936 |
| Au | 7.766241 | 14.220471 | 10.460131 |
| Au | 10.031064 | 14.080667 | 9.016945 |
| Au | 10.255827 | 13.443850 | 11.939808 |
| Au | 8.925831 | 11.747548 | 9.924155 |
| Au | 10.154661 | 7.622628 | 11.726768 |
| Au | 12.640514 | 8.220569 | 11.046215 |
